# Supplementary material for: Bulk superconductivity at 84 K in the strongly overdoped regime of cuprates
Source: arXiv:1612.04707 source file (2016-12-14)
Supplement: Supplementary file 1 [file Mo-cuprate-paper_SI.pdf]

# Supplementary information on the manuscript:

# Bulk superconductivity at 84 K in the strongly overdoped regime of cuprates

A. Gauzzi,[1,*] Y. Klein,[1] M. Nisula,[2] M. Karppinen,[2] P. K. Biswas,[3,†] H. Saadaoui,[3]
E. Morenzoni,[3] P. Manuel,[4] D. Khalyavin,[4] M. Marezio,[5] and T. H. Geballe[6]

[1]*IMPMC, Sorbonne Universités-UPMC, CNRS,*
*IRD, MNHN, 4, place Jussieu, 75005 Paris, France*

[2]*Aalto University, Department of Chemistry, Espoo 00076, Finland*

[3]*Laboratory for Muon Spin Spectroscopy,*
*Paul Scherrer Institut, CH-5232 Villigen PSI, Switzerland*

[4]*ISIS Facility, Rutherford Appleton Laboratory-STFC,*
*Chilton, Didcot, OX11 0QX, United Kingdom*

[5]*Institut Neél, CNRS and Université Grenoble Alpes, BP 166, 38042 Grenoble, France*

[6]*Stanford University, Department of Applied Physics*
*& Materials Science, Stanford CA 94305, USA*

(Dated: November 2, 2016)

In the present Supplementary Information section, we summarize the powder neutron diffraction (PND) results obtained on the $Cu_{0.75}Mo_{0.25}Sr_2YCu_2O_{7+\delta}$ powder sample studied by means of magnetization and specific heat measurements in the main text. The PND data have been collected at the high-resolution time-of-flight (TOF) WISH instrument[1], installed at the ISIS facility of the Rutherford Appleton Laboratory. For the present structural refinement, the diffracted profiles collected by the detector banks positioned at average $2\theta$ angles of 152.9°, 121.7° and 90° have been simultaneously employed using the Fullprof package[2]. A representative profile taken at 90° is shown in Fig. S1. In Tables 1-2, we report the refined structure, a summary of the refinement results and selected bond-length distances including the Cu-O apical one. The crystal structure is schematically represented in Fig. S2.

The main results of the present Rietveld refinement are as follows: (i) the molar purity of the $Cu_{0.75}Mo_{0.25}Sr_2YCu_2O_{7+\delta}$ powders is 95%, with 4.5% and 0.5% of KCl and $KClO_4$ impurities, respectively. The phases associated with a few minor peaks, barely visible in the profiles, were not identified. (ii) A high oxygen content, $\delta = 0.54$. (iii) A record short Cu-O apical distance of 2.165 Å. Point (i) supports the conclusion of bulk superconductivity presented in the main text, while points (ii) and (iii) confirm previous reports[3,4], thus enabling a direct comparison of the present study with the XANES results by Grigoraviciute *et al.*[3]

---

* Corresponding Author. E-mail:andrea.gauzzi@upmc.fr

† Present address: ISIS Facility, Rutherford Appleton Laboratory-STFC, Chilton, Didcot, OX11 0QX, United Kingdom.

1 L. C. Chapon, P. Manuel, P. G. Radaelli, C. Benson, L. Perrott, S. Ansell, N. J. Rhodes, D. Raspino, D. Duxbury, E. Spill, and J. Norris, Neutron News **22**, 22 (2011), http://dx.doi.org/10.1080/10448632.2011.569650.

2 J. Rodríguez-Carvajal, Physica B: Condensed Matter **192**, 55 (1993).

3 I. Grigoraviciute, M. Karppinen, T.-S. Chan, R.-S. Liu, J.-M. Chen, O. Chmaissem, and H. Yamauchi, J. Am. Chem. Soc. **132**, 838 (2010).

4 O. Chmaissem, I. Grigoraviciute, H. Yamauchi, M. Karppinen, and M. Marezio, Phys. Rev. B **82** (2010), 10.1103/PhysRevB.82.104507.

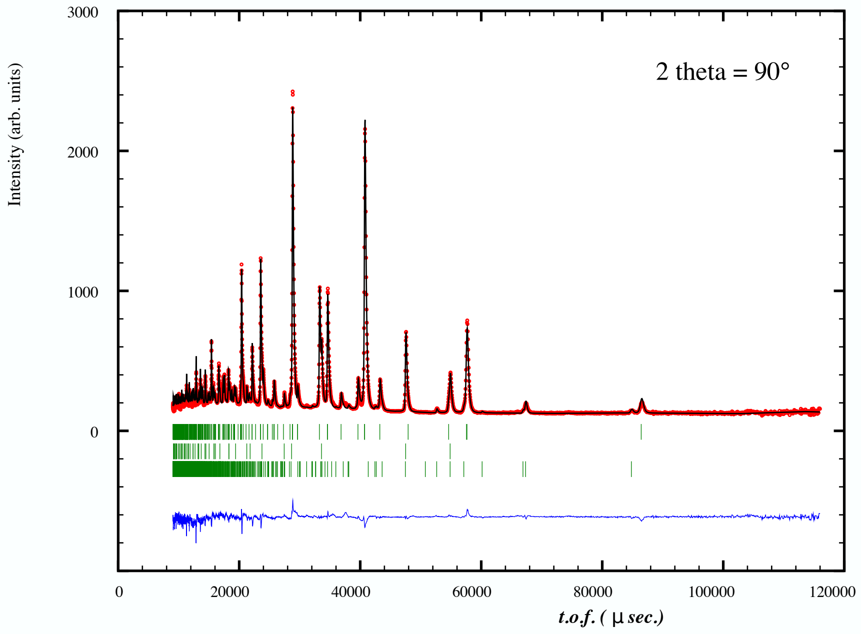


FIG. 1. TOF powder neutron diffraction profile taken by the 90° detector bank. Red points and black lines indicate the experimental and calculated profiles, respectively. Their difference is shown by the blue line. Green vertical ticks indicate the calculated position of the Bragg reflections for the main phase, $Cu_{0.75}Mo_{0.25}Sr_2YCu_2O_{7+\delta}$ (top), and for the two impurity phases, KCl (middle), and $KClO_4$ (bottom).

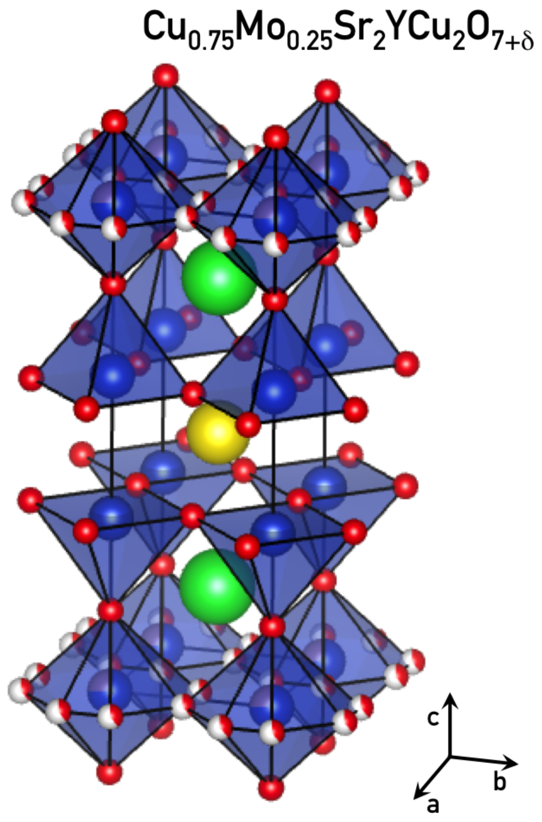


FIG. 2. Schematic representation of the tetragonal $P4/mmm$ structure of $Cu_{0.75}Mo_{0.25}Sr_2YCu_2O_{7+\delta}$. Blue, red, green and yellow spheres indicate Cu, O, Sr and Y atoms, respectively. Pink/blue spheres in the basal plane indicate the Cu1 site partially occupied by Mo. White/red spheres indicate the partially occupied O3 site, which determines the oxygen concentration, $\delta$. See also Table 1.

TABLE I. Rietveld refinement of the the tetragonal $P4/mmm$ structure of $Cu_{0.75}Mo_{0.25}Sr_2YCu_2O_{7+\delta}$ obtained from TOF powder neutron diffraction data taken at 300 K. Numbers in parentheses indicate statistical uncertainty. Refined lattice parameters are: $a = b$ = 3.81278(5) Å, $c$ = 11.45487(24) Å. Atomic coordinates, $x$, $y$, and $z$, are given in reduced lattice units. The values in Å of the isotropic thermal factors, $B_{\rm iso}$, are multiplied by 100. SOF indicates the site occupancy factor.

| Atomic site | Wyckoff position | $x$ | $y$ | $z$ | $B_{\rm iso}$ | SOF |
|---|---|---|---|---|---|---|
| Cu1 | 1a | 0 | 0 | 0 | 1.396(89) | 0.75 |
| Mo1 | 1a | 0 | 0 | 0 | 1.396(89) | 0.25 |
| Sr1 | 2h | 0.5 | 0.5 | 0.18338(23) | 2.152(72) | 1 |
| Cu2 | 2e | 0 | 0 | 0.35435(19) | 0.768(47) | 1 |
| Y1 | 1d | 0.5 | 0.5 | 0.5 | 1.429(88) | 1 |
| O1 | 2g | 0 | 0 | 0.16537(29) | 1.666(115) | 1 |
| O2 | 4i | 0.5 | 0 | 0.37491(16) | 1.367(61) | 1 |
| O3 | 4n | 0.5 | 0.11614(166) | 0 | 3.451(217) | 0.3854(37) |

Reliability factors for the profiles taken at $2\theta$=152.9°, 121.7°, and 90° were as follows:
$R_p$=2.97, 4.92, and 5.10 and $R_{wp}$=3.18, 4.59, and 4.29, respectively.

TABLE II. Cu- and Mo-O bond-length distances in Å and buckling angle of the $CuO_2$ plane in °. Numbers in parentheses indicate statistical uncertainty.

| Atoms | Distance | Angle |
|---|---|---|
| Cu1(Mo1)-O1 | 1.957(6) | |
| Cu1(Mo1)-O3 | 1.894(3) | |
| Cu2-O1 | 2.165(4) | |
| Cu2-O2 | 1.9209(4) | |
| O2-Cu2-O2 | | 165.9(2) |
